# Supplementary material for: Spatiotemporal-aware Trend-Seasonality Decomposition Network for Traffic Flow Forecasting
Source: arXiv:2502.12213 source file (2025-02-17)
Supplement: Supplementary file 1 [file supplement.tex]

\section{Supplement}

\subsection{Notations}

Key notations used in the paper and their definitions are summarized in Table~\ref{tab.notations}.

\begin{table}[http]
    \vspace{-2mm}
    \begin{center}
    % \vspace{-2mm}
    % \fontsize{9}{12} \selectfont
    \setlength{\tabcolsep}{1mm}{}	
    \begin{tabular}{c|c}
        \toprule
        Notation  & Definition \\
        \hline
        $\mathcal{G}$ & the input traffic network\\
        $\mathcal{V}$ & the node set of $\mathcal{G}$ \\
        $\mathcal{E}$ & the edge set of $\mathcal{G}$ \\
        $T$ & length of input traffic signal matrix tensor\\
        $T^\prime$ & length of output traffic signal tensor\\
        $N$ & number of monitor nodes \\
        $C$ & number of observed features \\
        $L$ & number of BT blocks in decoder \\
        \hline
        $\mathbf{A}$ & the input adjacent matrix \\
        $\mathbf{X}_{t}$ & traffic signal matrix at time slice $t$ \\
        $\bm{\mathcal{X}}$ & the input traffic signal tensor \\
        $\bm{\mathcal{\hat{X}}}$ & the expected traffic signal tensor \\
        \hline
        $\bm{\mathcal{A}}$ & the constructed dynamic relaionship graph \\
        $\bm{\mathcal{H}}_L$ & output of dynamic relationship graph learning \\
        $\mathbf{M}^{t}_{h}$ & the historical temporal embedding \\
        $\mathbf{M}^{t}_{h}$ & the predicted time embedding \\
        $\mathbf{M}^{s}$ & the spatial embedding \\ 
        $\bm{\mathcal{M}}$ & the spatio-temporal embeddings \\
        $\bm{\mathcal{X}}_{s}$ & the seasonal part of sequence data \\
        $\bm{\mathcal{X}}_{t}$ & the trend-cyclical part of sequence data \\
        \hline
        $\bm{\mathcal{Y}}$ & the output of encoder \\
        $\bm{\mathcal{H}}$ & input of the BT block in encoder \\ 
        $\mathbf{IT}$ & reference points of the BT block \\
        $\bm{\mathcal{Z}}$ & output of the BT block \\
        \bottomrule
    \end{tabular}
    \vspace{-2mm}
    \caption{Main notations and their definitions. Calligraphic symbols denote 3D tensors.}
    \vspace{-6mm}
    \label{tab.notations}
    \end{center}
\end{table}

\subsection{Datasets}

The PeMS04 and PeMS07 datasets are collected bu the Caltrans Performance Measurement System (PeMS). They are made to public datasets by \cite{song2020STSGCNaaai}.

The JiNan dataset is collected in a real-world city in China. The traffic flow data has been meticulously aggregated into intervals of five minutes, resulting in a total of 288 discrete time steps within a single day. Additionally, within the spatial network model, two monitoring points are deemed interconnected if they are situated along the same road segment. Though we provide the distance between two nodes based on connectivity, we still do not recommend building the adjacency matrix based on distance. Given the intricacies of urban transportation networks, we opt to utilize a binary representation, with '1' indicating the presence of a connection, rather than encoding the distance. Figure~\ref{fig:JiNan} show the detail of JiNan dataset.

\begin{figure}[http]
    \centering
    \vspace{-2mm}
    \includegraphics[width=0.95\linewidth]{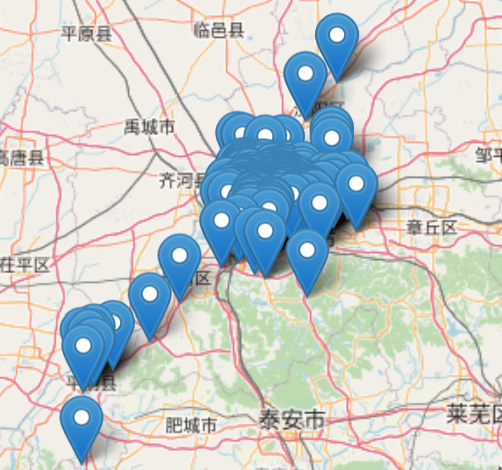}
    \caption{The detail of JiNan dataset.}
    \vspace{-6mm}
    \label{fig:JiNan}
\end{figure}

\subsection{Baselines}
The publicly source codes of baselines can be available at the following URLs:

% DCRNN: \url{https://github.com/chnsh/DCRNN_PyTorch}

% STGCN: \url{https://github.com/hazdzz/STGCN}

% GWNet: \url{https://github.com/nnzhan/Graph-WaveNet}

% GMAN: \url{https://github.com/zhengchuanpan/GMAN}

% ASTGCN: \url{https://github.com/guoshnBJTU/ASTGCN-2019-pytorch}

% AGCRN: \url{https://github.com/LeiBAI/AGCRN}

% DMSTGCN: \url{https://github.com/liangzhehan/DMSTGCN}
% STGODE: \url{https://github.com/square-coder/STGODE}
% STGNCDE: \url{https://github.com/jeongwhanchoi/STG-NCDE}
% D\textsuperscript{2}STGNN: \url{https://github.com/GestaltCogTeam/D2STGNN}
% DSTAGNN: \url{https://github.com/SYLan2019/DSTAGNN}
% SSTBAN: \url{https://github.com/guoshnBJTU/SSTBAN}
% STWave: \url{https://github.com/LMissher/STWave}
\begin{itemize}
    \item DCRNN: \url{https://github.com/chnsh/DCRNN_PyTorch}
    \item STGCN: \url{https://github.com/hazdzz/STGCN}
    \item GWNet: \url{https://github.com/nnzhan/Graph-WaveNet}
    \item GMAN: \url{https://github.com/zhengchuanpan/GMAN}
    \item ASTGCN: \url{https://github.com/guoshnBJTU/ASTGCN-2019-pytorch}
    \item AGCRN: \url{https://github.com/LeiBAI/AGCRN}
    \item DMSTGCN: \url{https://github.com/liangzhehan/DMSTGCN}
    \item STGODE: \url{https://github.com/square-coder/STGODE}
    \item STGNCDE: \url{https://github.com/jeongwhanchoi/STG-NCDE}
    \item D\textsuperscript{2}STGNN: \url{https://github.com/GestaltCogTeam/D2STGNN}
    \item DSTAGNN: \url{https://github.com/SYLan2019/DSTAGNN}
    \item SSTBAN: \url{https://github.com/guoshnBJTU/SSTBAN}
    \item STWave: \url{https://github.com/LMissher/STWave}
\end{itemize}
% DMSTGCN: \url{https://github.com/liangzhehan/DMSTGCN}
Besides that, you can get a more standardized and summarized code at the following URLs:
\begin{itemize}
    \item LargeST: \url{https://github.com/liuxu77/LargeST}
    \item FlashST: \url{https://github.com/HKUDS/FlashST}
\end{itemize}
In the meanwhile, our code is available at \url{https://anonymous.4open.science/r/mycode-FB23}

\subsection{Additional Experiments}
To evaluate the importance of spatial embedding and temporal embedding, we set $\alpha$ to be the trainable parameters. Similar with the equation~\ref{eq:embeddings}, we change it to:

\begin{equation}
    \bm{\mathcal{M}} = \alpha\sigma_{1}(\bm{\mathcal{M}}^{t}_{h}) + (1-\alpha)\sigma_{2}(\bm{\mathcal{M}}^{s}).
\end{equation}

The initial value of $\alpha$ is designated as 0.5, and the experimental results on PeMS04 dataset are shown in Table~\ref{tab.addi}. The findings do not surpass the performance of \model, leading us to hypothesize that rudimentary parameter configurations may not adequately capture the nuanced influence that distinct embeddings exert on the dataset. It is suggested that a more sophisticated parameter tuning process is required to fully realize the potential of the embedding mechanisms within the model's predictive capabilities.

In the meanwhile, we set $\beta$ as the trainable parameters to evaluate the importance of trend-cyclical part and seasonal part:
\begin{equation}
    \bm{\mathcal{Y}} = \beta\bm{\mathcal{Y}}_{t} + (1-\beta)\bm{\mathcal{Y}}_{s}.
\end{equation}

% The parameter $\beta$ is initialized at a value of 0.5, and the experimental results on PeMS04 dataset are shown in Table~\ref{tab.addi}. The result is not better than \model. The observed results do not outperform the performance of \model. This observation prompts us to surmise that the simplicity of our initial parameter settings may not sufficiently encapsulate the profound effects that parameter variations can have on the dataset. It is our conjecture that a more nuanced approach to parameter tuning is imperative to accurately reflect and leverage the impact of these settings on the data's predictive modeling efficacy. The incorporation of additional parameters could have inadvertently amplified the noise within the model, which in turn has led to a considerable reduction in the quality of the results. This suggests that the complexity introduced by these parameters may have outweighed their potential benefits, resulting in a less effective model. It highlights the need for a judicious balance in parameter selection to ensure that the model remains sensitive to meaningful data patterns without being overwhelmed by noise.

The parameter $\beta$ was set to 0.5 for our experiments on the PeMS04 dataset, with results detailed in Table~\ref{tab.addi}. However, these results did not surpass the performance of \model. It seems that our straightforward initial parameter choice did not capture the full impact of parameter variations on the data. We believe that a more refined parameter tuning process is necessary to enhance the model's predictive power. The addition of extra parameters may have actually increased noise, degrading the model's performance. This indicates that while more parameters can be beneficial, they must be carefully managed to avoid overwhelming the model with unnecessary complexity and noise.

\begin{table}[http]
    \vspace{-2mm}
    \begin{center}
    % \vspace{-2mm}
    % \fontsize{9}{12} \selectfont
    \setlength{\tabcolsep}{3mm}{}	
    \begin{tabular}{cccc}
        \toprule
        \textbf{Model}&MAE&RMSE&MAPE\\
        \hline
        \text{with $\alpha$} &19.06	&31.43	&12.66\% \\
        \text{with $\beta$} &19.10	&31.53	&12.39\% \\
        \text{\model} & 18.40 & 30.41 &12.21\% \\
        % \text{SD} & 716 & 17,319 & 15\text{min} & 01/2019-12/2019 \\
        % \text{GBA} & 2,352 & 61,246 & 15\text{min} & 01/2019-12/2019 
        \bottomrule
    \end{tabular}
    \vspace{-2mm}
    \caption{Additional experiments on PeMS04 dataset.}
    \vspace{-6mm}
    \label{tab.addi}
    \end{center}
\end{table}

\subsection{Algorithm Pseudo-Code}
Algorithm~\ref{alg:algorithm} shows the pseudo-code of our proposed \model.

\begin{algorithm}[http]
\caption{The Learning Process of \model}
\label{alg:algorithm}
\textbf{Input}: Input traffic nwtwork $\mathcal{G}$, historical traffic values $\bm{\mathcal{X}}$, the time of day $\mathbf{z}^{d}$ and the day of week $\mathbf{z}^{w}$\\
% \textbf{Parameter}: Optional list of parameters\\
\textbf{Output}: Predicted traffic values $\bm{\mathcal{\hat{X}}}$
\begin{algorithmic}[1] %[1] enables line numbers
\STATE Construct the dynamic relationship graph $\bm{\mathcal{A}}$
\STATE Calculate the processed sequence data $\bm{\mathcal{H}}_L$
\STATE Calculate the spatio-temporal embeddings $\bm{\mathcal{M}}$ 
\STATE Generate the trend-cyclical part of sequence data $\bm{\mathcal{X}}_{t} = \bm{\mathcal{H}}_L \odot \bm{\mathcal{M}}$
\STATE Generate the seasonal part of sequence data $\bm{\mathcal{X}}_{s} = \bm{\mathcal{H}}_L - \bm{\mathcal{X}}_{t}$
\STATE Get the processed trend-cyclical component by GRU encoder $\bm{\mathcal{Y}}_{t} = GRU(\bm{\mathcal{X}}_{t})$
\STATE Get the processed seasonal component by GRU encoder $\bm{\mathcal{Y}}_{s} = GRU(\bm{\mathcal{X}}_{s})$
\STATE Sum the two components $\bm{\mathcal{Y}} = \bm{\mathcal{Y}}_{t} + \bm{\mathcal{Y}}_{s}$
\FOR{$i$ = 1 to $L$}
\STATE Calculate $\bm{\mathcal{Z}}^{l}$ in the $l$-th BT block 
\ENDFOR
\STATE Calculate expected traffic predictions $\bm{\mathcal{\hat{X}}}$ by a fully-connected neural network
\STATE Calculate $\mathcal{L}$ using equation~\ref{eq:loss}
\STATE Back propagation and update parameters in \model
\STATE Return $\bm{\mathcal{\hat{X}}}$
\end{algorithmic}
\end{algorithm}
